# Supplementary material for: Precise Event Spotting in Sports Videos: Solving Long-Range Dependency and Class Imbalance
Source: arXiv:2503.00147 source file (2025-02-28)
Supplement: Supplementary file 1 [file X_suppl.tex]

\clearpage
\setcounter{page}{1}
\maketitlesupplementary

This supplementary presents the following details which we could not include in the main paper due to space constraints:
\tableofcontents

\begin{figure*}[!t]
\subfloat[SoccerNet V2 dataset \cite{SoccerNetv2}]{\centering
    \includegraphics[width=0.99\textwidth]{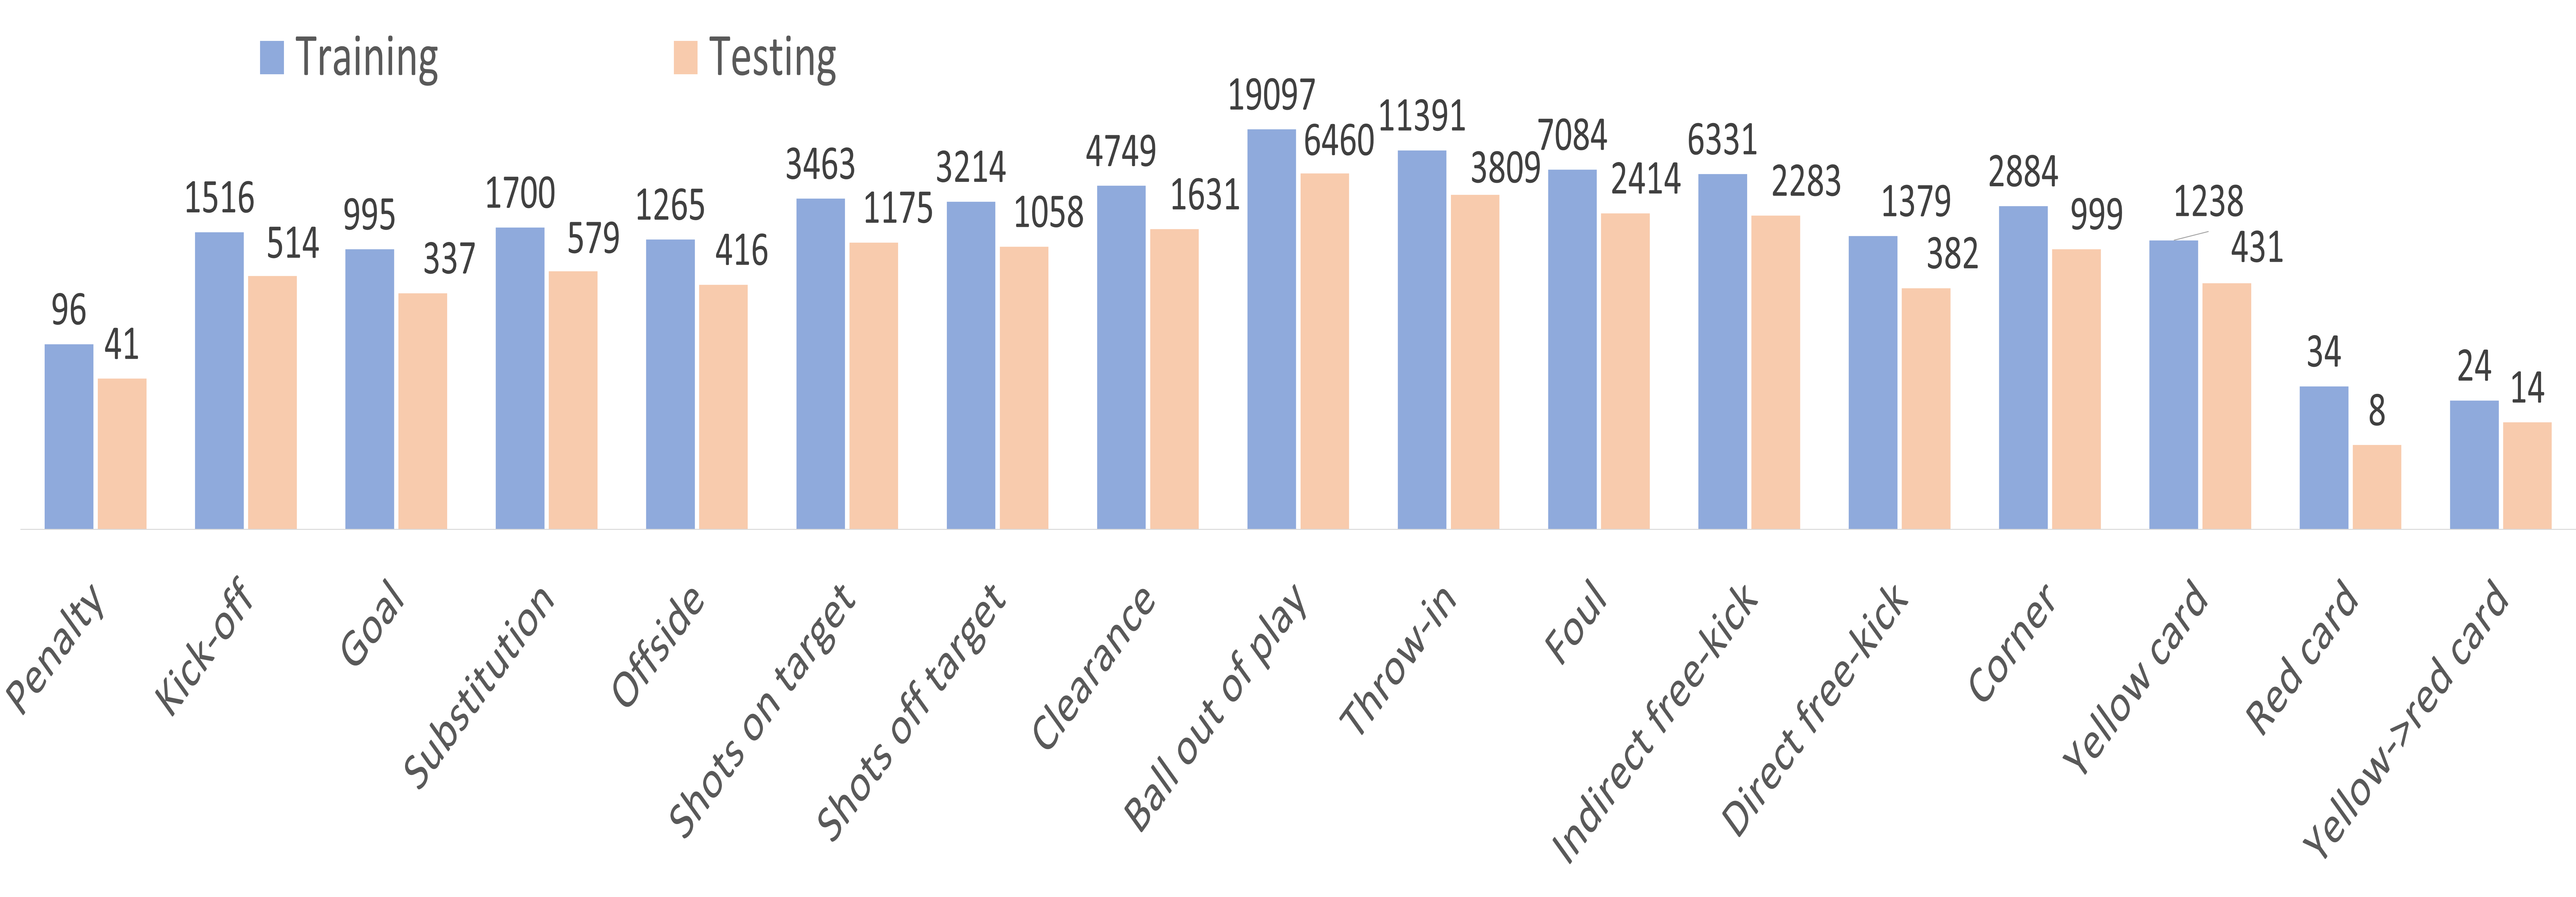}} \\
\subfloat[Tennis dataset \cite{vid2player}]{\centering
    \includegraphics[width=0.33\textwidth]{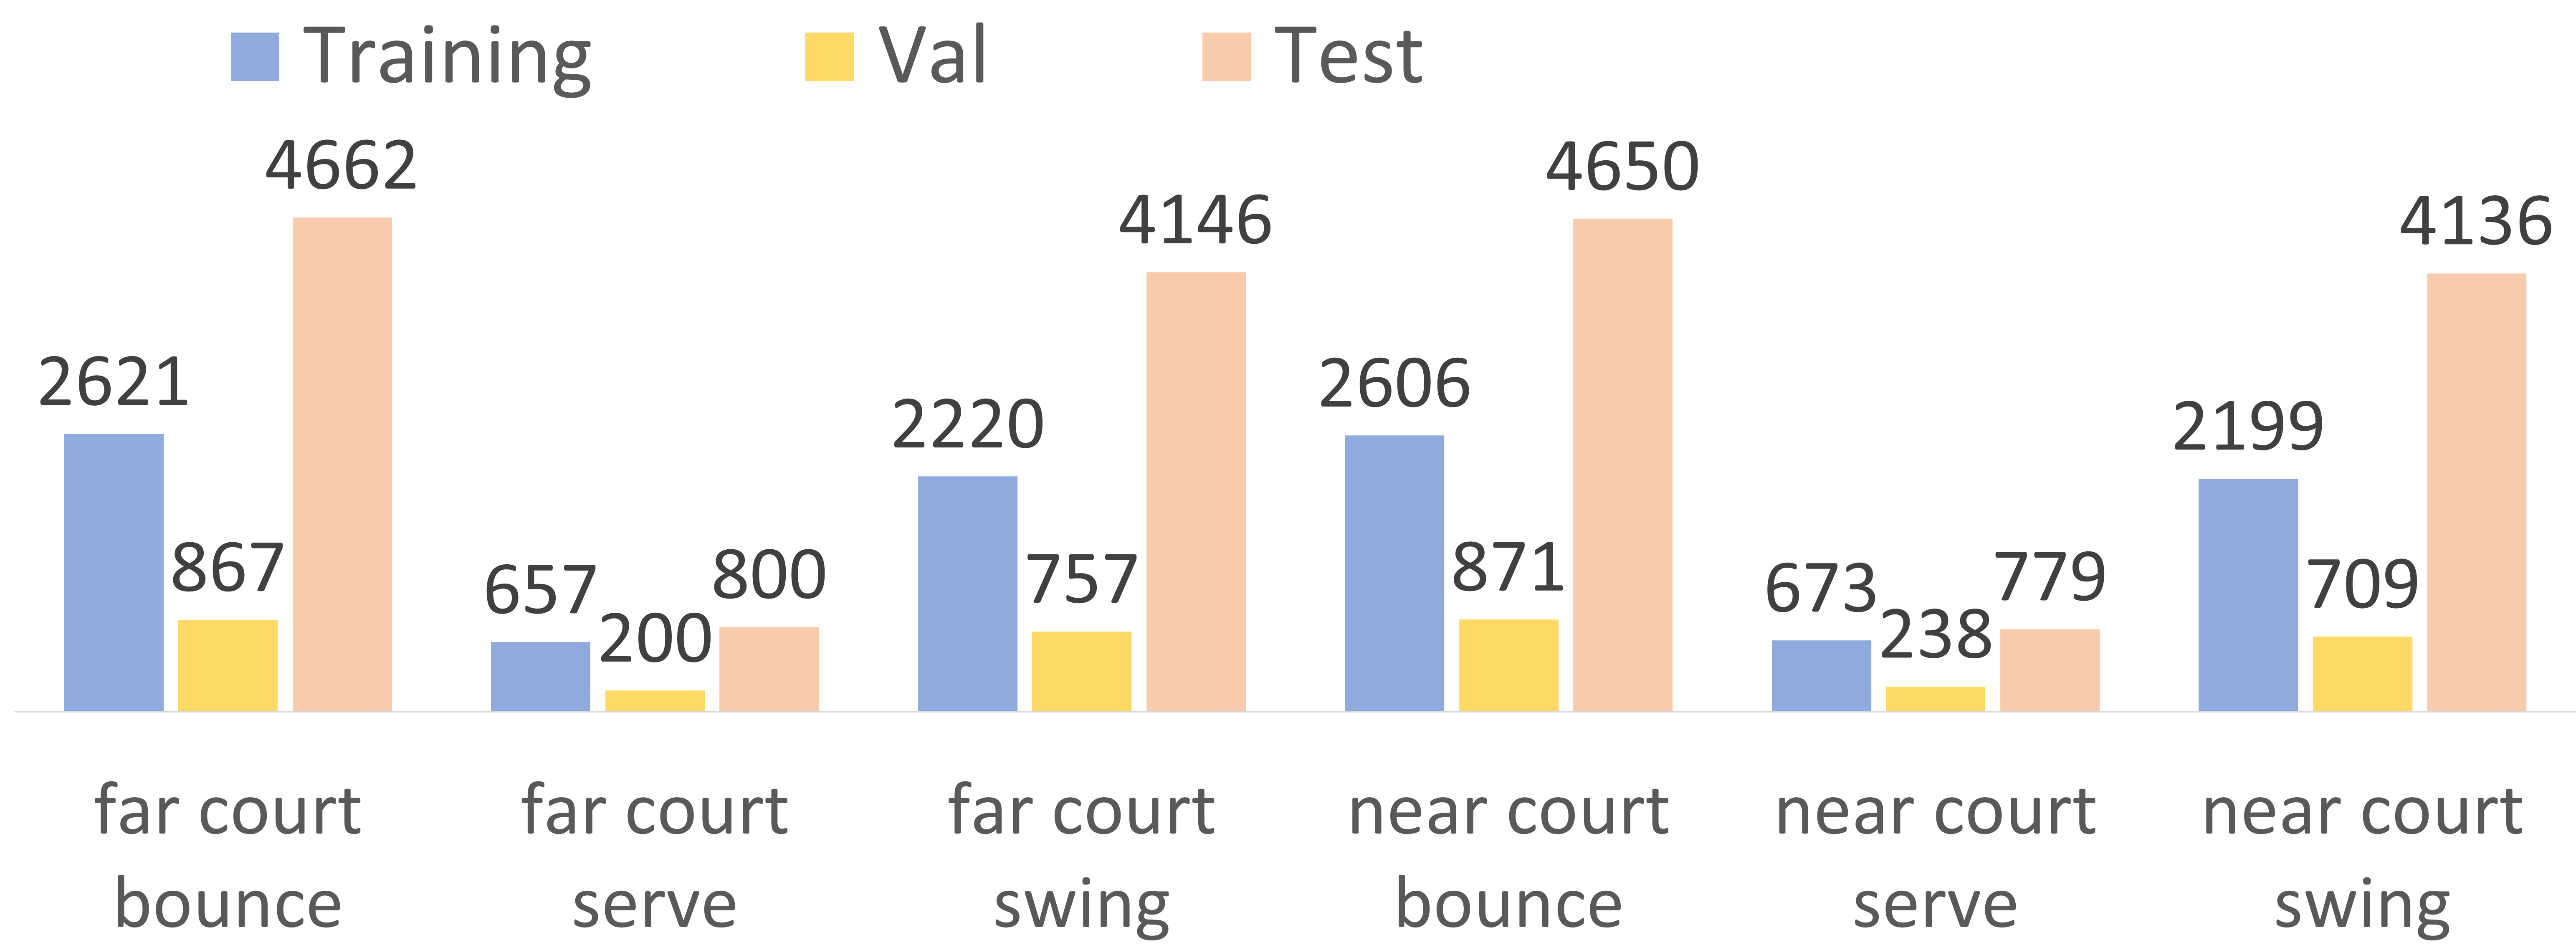}} \hfill
\subfloat[FS-Comp dataset \cite{fs}]{\centering
    \includegraphics[width=0.33\textwidth]{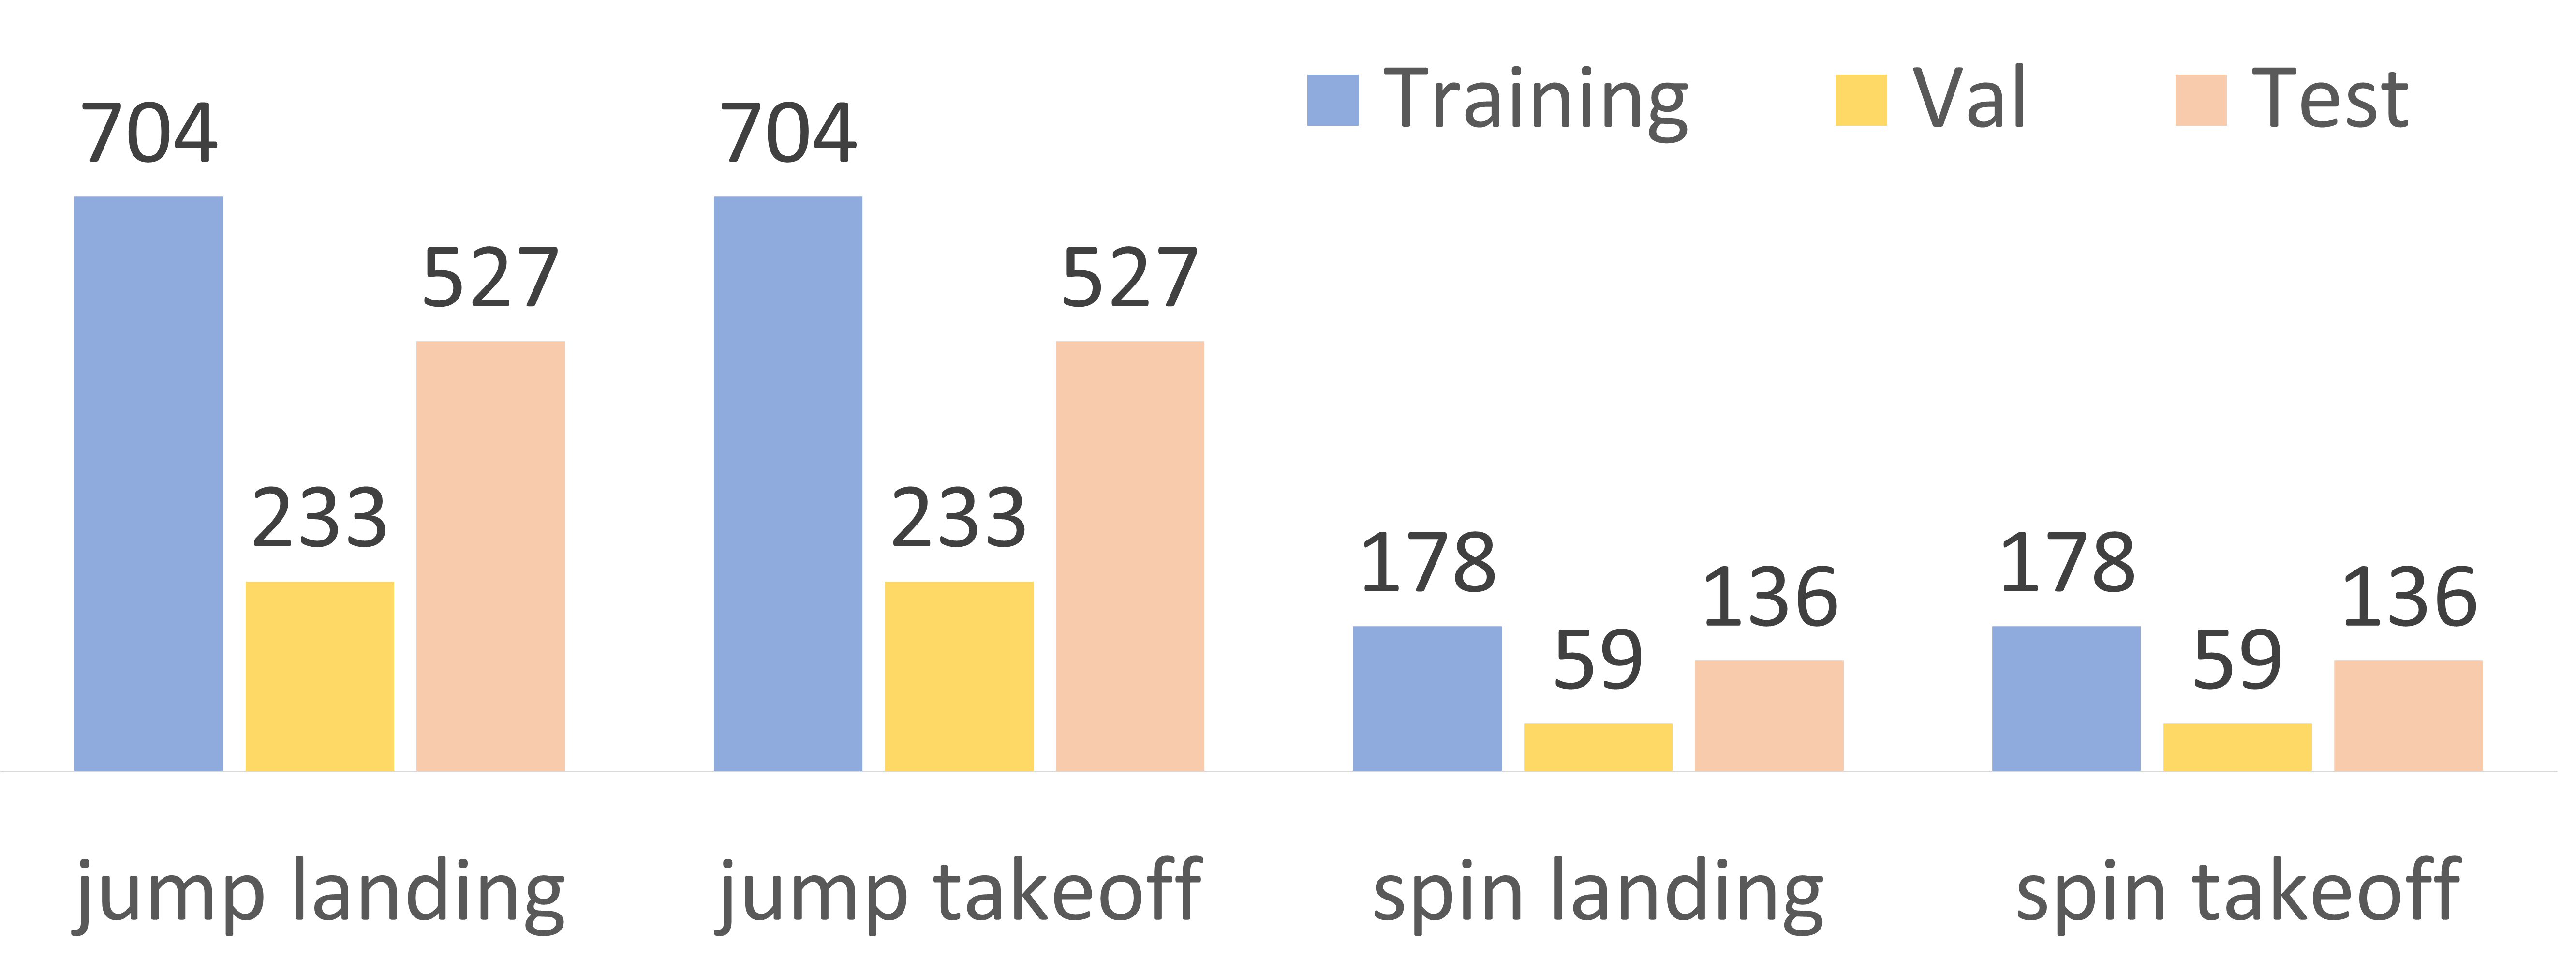}} \hfill
\subfloat[FS-Perf dataset \cite{fs}]{\centering
    \includegraphics[width=0.33\textwidth]{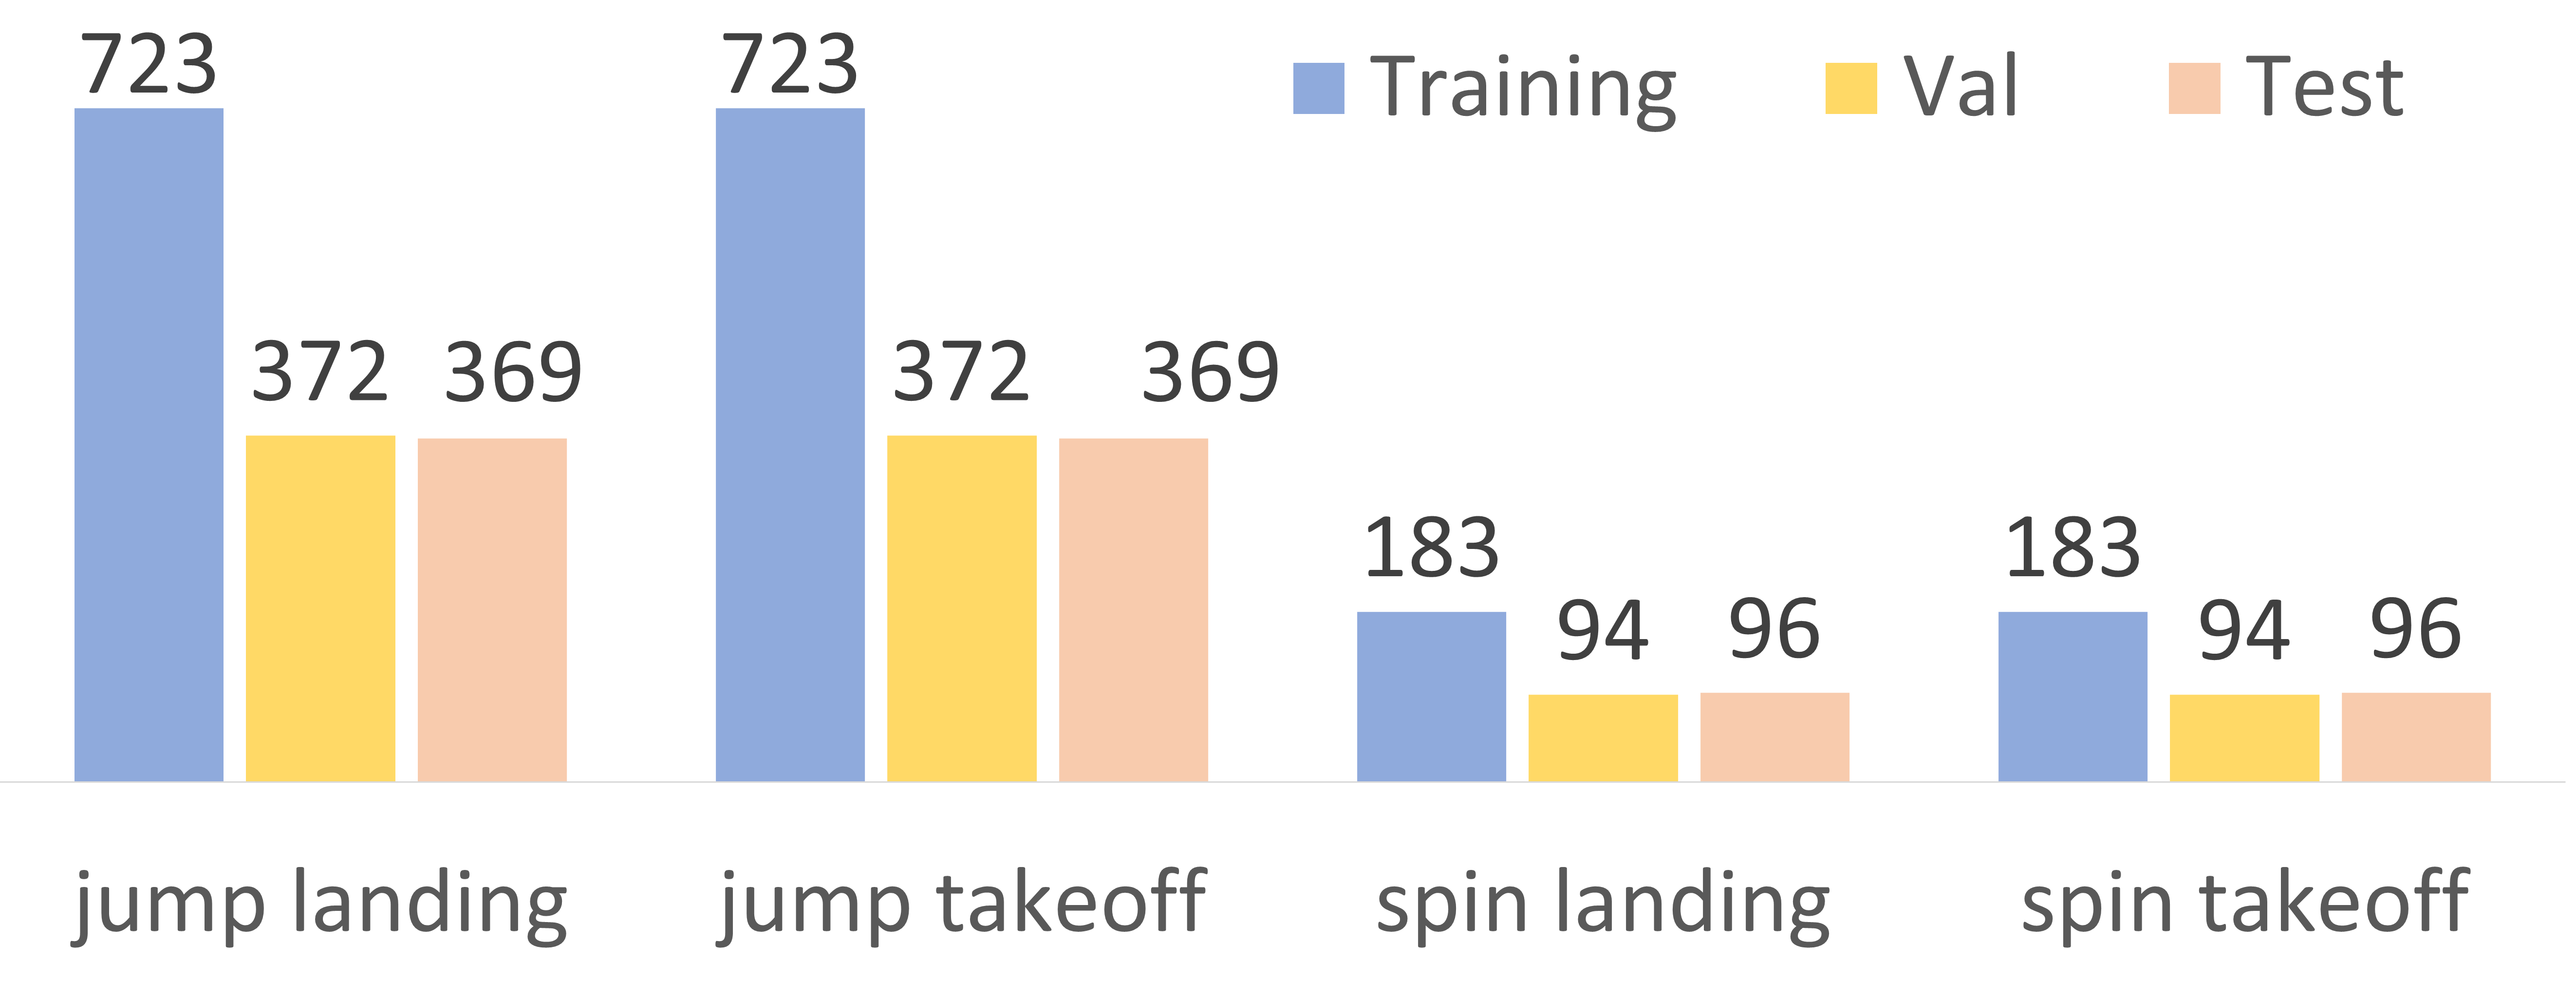}} \\
\subfloat[FineGym dataset \cite{finegym}.  This dataset has total 32 classes, apart from `VT' classes, all other classes have same number of start and end events. So, here we show the `start' events only.]{\centering
    \includegraphics[width=0.99\textwidth]{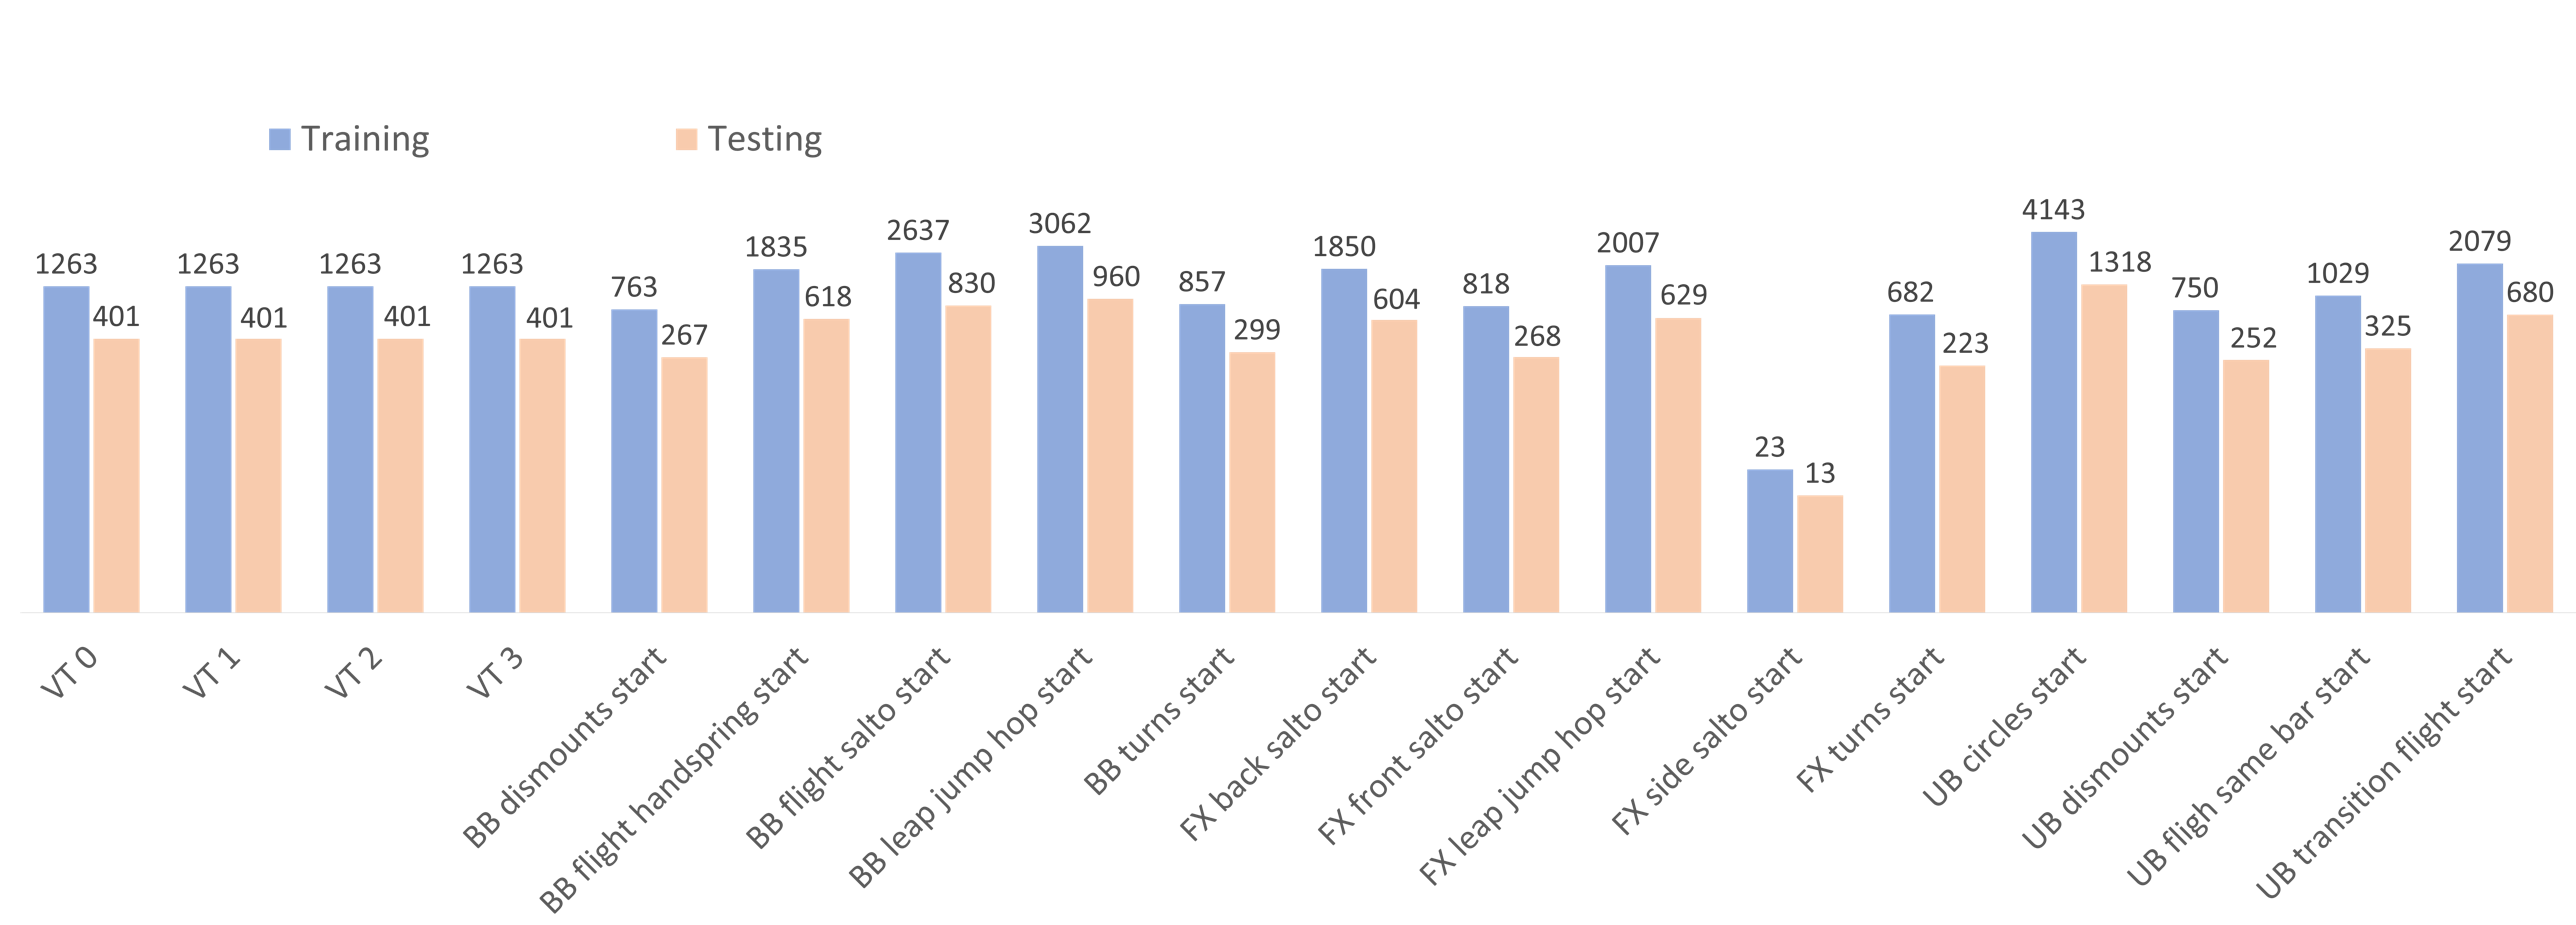}}
    \caption{Class-wise distributions of SoccerNet V2, Tennis, Figure Skating (i.e., FS-Comp \& FS-Perf) and FineGym datasets.} \label{fig:tennis_skating_dataset}
\end{figure*}

\section{ Dataset \& Implementation Details}\label{{sup:dataset}}
\subsection*{Dataset Description}
We have utilized event spotting datasets like Tennis~\cite{vid2player}, Figure Skating (FS)~\cite{fs}, FineGym~\cite{finegym} and the SoccerNet V2~\cite{SoccerNetv2} action spotting dataset to evaluate our method. Below we provide the details of these datasets.

% To validate the efficacy of the proposed method, we have conducted experiments using event spotting datasets outlined in~\cite{e2espot} such as Tennis~\cite{vid2player}, Figure Skating (FS)~\cite{fs}, Fine Gym and the SoccerNet V2~\cite{SoccerNetv2} action spotting dataset. Details of these datasets are as follows:

\noindent\textbf{SoccerNet V2}~\cite{SoccerNetv2} is a large-scale dataset of soccer videos containing 764 hours of data from 500 games, annotated for tasks like action spotting, camera shot segmentation and boundary detection, and replay grounding. We have utilized the action spotting dataset, which designates 17 different actions as events. This data is processed at 2 FPS. Each action of this dataset is annotated with a single timestamp as per the well-established soccer rules. 
% Annotation details can be found in \cite{SoccerNetv2}. 
There are 110,458 annotations, averaging one action every 25 seconds. Due to the nature of events, there is an inherent imbalance among the classes. For example, card events are much less likely to occur than other events like fouls or throw-ins. As it can be seen  Figure~\ref{fig:tennis_skating_dataset} (a),  ``Red Card'' and ``Yellow\textrightarrow Red Card'' have only a few samples, while the ``Ball out of play'' class has thousands of samples. 
% Additionally, a visibility tag is associated with each action: \emph{shown} or \emph{unshown}. \emph{Shown} means the action is shown in the broadcast video and in the \emph{unshown} case, the action is not explicitly shown but needs to be inferred from the context, such as during a goal replay the following kick-off may not always be shown.

\noindent \textbf{Tennis} dataset, compiled by \cite{e2espot}, is an extension of the dataset proposed in Vid2Player~\cite{vid2player}. It contains 3345 clips from 28 tennis matches (9 original + 19 new) from Wimbledon and US Open tournaments. The videos are either 25 or 30 FPS frames. 19 videos were used for training and validation, whereas the remaining 9 were kept for testing. The events are categorized into six classes: ``Player serve ball contact", ``regular swing ball contact" and ``ball bounce" for near- and far-court. Out of the 1.3M frames in the dataset, only 33,791 frames (2.6\%) contain precise temporal events. Imbalance can also be seen in this dataset; ``Serve'' event (both far count and near court)  has significantly fewer samples than other actions (Figure~\ref{fig:tennis_skating_dataset} (b)).

\noindent\textbf{Figure Skating} (FS)~\cite{fs} dataset contains 11 videos featuring performances from the Winter Olympics (2010-2018) and World Championships (2017-2019). All videos are 25 FPS. The original labels have been re-annotated by \cite{e2espot} considering four actions: take-off and landing frames of jump and flying spins. In this dataset also, the sample count is not uniform; both ``Spin'' events has significantly less number of samples compared to the ``Jump'' event (Figure~\ref{fig:tennis_skating_dataset} (c-d)). Two splits of this dataset are considered for evaluation:
\begin{itemize}
    \item \textbf{Competition Split (FS-Comp)}: All the videos from the 2018 season are kept for testing. So, the generalization capability of the methods to unseen videos (for example, change in background) could be evaluated. 
    \item \textbf{Performance Split (FS-Perf)}: In this split, each competition is stratified across train, validation and test. This mainly evaluates the performance of the method when the skater changes without the unseen background situation.
\end{itemize}

\noindent \textbf{FineGym}~\cite{finegym} dataset contains 5,374 gymnastics performances and each of them is treated as an untrimmed video. It has 32 classes, derived from a hierarchy of action categories (e.g., balance beam dismount; balance beam turns). The original annotations denote the start and end of the actions; but here these boundaries are considered as events: “balance beam dismount start” and “balance beam dismount end”. Original splits are designed for action recognition, so are using the split proposed by the \cite{e2espot} for the action spotting task. There are variations in the input video frame rates, so 50 and 60 FPS videos are resampled to 25 and 30 respectively. In this dataset only ``FX side salto'' event have less number of samples, while all other events have sufficiently large number of samples (Figure~\ref{fig:tennis_skating_dataset} (e)).

\subsection*{ Implementation Details}   
In addition to the implementation details provided in Subsection 4.1 in the main manuscript, here we have provided additional details of the proposed model applied to training on different datasets. In one training epoch, we sample a fixed number of clips from each video. During testing, samples are taken using a sliding window of 128 frames with a 50\% overlap. Due to that, the sample size of each epoch varies from dataset to dataset. During the training process, a few configurations differ for each dataset. Below are the specific changes in the training configuration for each dataset:
\begin{itemize}
    \item SoccerNet V2: The training data is sampled uniformly at random without overlap. Fifty clips are sampled from each video in one epoch. During training, the proposed model is trained up to 120 epochs. The frames are processed at $398\times224$ without cropping, as cropping may result in the loss of events occurring on the edges of the frame.
    \item Tennis: The training data is sampled at uniform random. Four clips are sampled from each video in one epoch. Similar to the SoccerNet V2 dataset, the frames are processed at $398\times224$ without cropping. Here, the model is trained for 100 epochs. 
    \item Figure Skating: The training data is sampled at uniform random. Ten clips are sampled from each video in one epoch. Training is conducted using frames cropped to $224\times224$. We have observed that using non-cropped frames results in increased computation without improvement in the spotting accuracy. Here, the model is trained for 300 epochs. The exact same configuration has been utilized in both FS-Comp and FS-Perf.
    \item FineGym: In FineGym also, the training data is sampled at uniform random taking 10 clips at a time from each video. The model is trained with random crops of $224\times 224$, while during testing we center crop the video to $224\times 224$. The model is trained for 100 epochs. 
\end{itemize}
In all datasets, the model is trained on multiple GPUs with a batch size of 2 at each GPU. The best-performing model is chosen based on the score in the validation dataset, and the same model generates the results. Additionally, we use the Soft-NMS with a window size of 20 to process the results. 

We reproduce the results from the author provided checkpoint of E2E-Spot\footnote{https://github.com/jhong93/spot}, COMEDIAN\footnote{https://github.com/juliendenize/eztorch}, UGLF\footnote{https://github.com/Fsoft-AIC/UGLF} and T-DEED\footnote{https://github.com/arturxe2/T-DEED} methods only when the corresponding results are not provided in their respective paper.

\begin{table}[t!]
\centering
\caption{Analysis of various Temporal networks on Tennis~\cite{vid2player} dataset test set. The metric of comparison is \textbf{mAP}.} \label{tab:Spotting-Head}
% \small
\begin{adjustbox}{max width=0.8\linewidth}
\begin{tabular}{@{}lccc@{}}
\toprule
\multirow{2}{*}{Method} & \multicolumn{3}{c}{Tennis} \\ \cmidrule{2-4}
  & $\delta$ = 0   & $\delta$ = 1   & $\delta$ = 2    \\
\midrule
Baseline with Bi-GRU &   45.34   & 96.10   & 97.70  \\
\rowcolor{lightmintbg} Proposed with Bi-GRU  &  \textbf{61.01}   & \textbf{96.21}   & \textbf{97.75} \\
\quad with Deformable Attention  &    53.71  & 88.50   &  97.33  \\
\quad with Bi-GRU 2 Layers  &   51.22  & 88.42  &  97.44  \\
\quad with Transformer (L1H8)   & 52.83   & 89.23   & 97.10   \\
\quad with Transformer (L2H8)   &  52.89  &  90.49  &  96.95  \\
\quad with Bi-LSTM  &  52.54   & 88.06   & 97.63   \\
\quad with MSTCN  & 59.90    & 95.26   & 97.37  \\
\bottomrule
\end{tabular} 
\end{adjustbox}
\end{table}

\begin{table}[t!]
\small
\centering
\caption{Efficiency Comparison in terms of GFLOPs and number of parameters of the proposed and recent SOTA methods. * indicate that the GFLOPs value is calculated from the temporal network only without feature extractors. Here, ASTRA model utilized the features extracted from Baidu model which is made up of 5 large networks.}
\label{tab:efficiency}
\begin{adjustbox}{max width=0.9\linewidth}
\begin{tabular}{lccc}
\toprule
Methods                   & GFLOPs & \begin{tabular}[c]{@{}c@{}} \# of Parameters \\ (in Millions)\end{tabular} \\
\midrule
E2E-Spot (RegNet-Y 200MF) &   39.61     &  4.46         \\
E2E-Spot (RegNet-Y 800MF) &   151.4     &    12.64         \\
ASTRA                     &   8.83*     &      44.33       \\
Spivak                     &   461.89     &    17.46     \\
% UGLF                  &   39.61     &   4.46   \\
COMEDIAN (ViSwin)                &   222.76    &     70.12   \\
T-DEED (RegNet-Y 200MF)   &    21.96    &    16.36    \\
T-DEED (RegNet-Y 800MF)   &      85.58  &   46.22   \\
\rowcolor{lightmintbg} Proposed  &  60.25  &  6.46     \\
\bottomrule
\end{tabular}
\end{adjustbox}
\end{table}

%%%%%%%%%%%%%%%%%%%%%%%%%%% Spotting Head Analysis on Tennis Dataset %%%%%%%%%%%%%%%%%%%%%%%%%%%
\section{ Analysis on Different Temporal modules}
In our proposed approach, we opted for the bidirectional GRU (Bi-GRU) as the long-range dependency module in the temporal block. %  after conducting various experiments with different potential temporal networks. 
In the main paper we have shown the results obtained from using different networks on the SoccerNet V2~\cite{SoccerNetv2} dataset. Here, in Table~\ref{tab:Spotting-Head} we present the results obtained from on Tennis~\cite{vid2player} dataset. The results are in line with what we have already observed in the main paper: there is significant improvement in the scores across all the tolerances. Compared to the baseline method of E2E-Spot~\cite{e2espot} which also uses Bi-GRU as the temporal module, there is an improvement of 15.67\% in $\delta=0$ setting on the Tennis dataset. This reiterates the importance of the proposed ASTRM module and SoftIC Loss function.
% The results indicate that the Bi-GRU, as a temporal network, performs favorably compared to other temporal networks. Even more advanced temporal networks, such as and Bi-LSTM, Transformer heads, Deformable Attention~\cite{tadtr} and MSTCN~\cite{ms-tcn}, could not surpass the scores achieved by the Bi-GRU temporal network. The difference in scores is visible across all tolerances.  
% It is also observed that the proposed method generates significantly better results than the baseline E2E-Spot method, which also uses Bi-GRU as the temporal block. For instance, the proposed method achieves a 12.55\% and 5.86\% improvements over baseline model in the tight and loose settings of SoccerNet V2 dataset, respectively. Similarly, there is an improvement of 15.67\% in $\delta=0$ setting compared to baseline on Tennis dataset. 
% Here, this significant improvement is attributed to the proposed ASTRM module and the proposed SoftICLoss function.
% which helps the proposed method to perform well especially in tight settings.
\begin{figure*}[t!]
    \includegraphics[width=\textwidth]{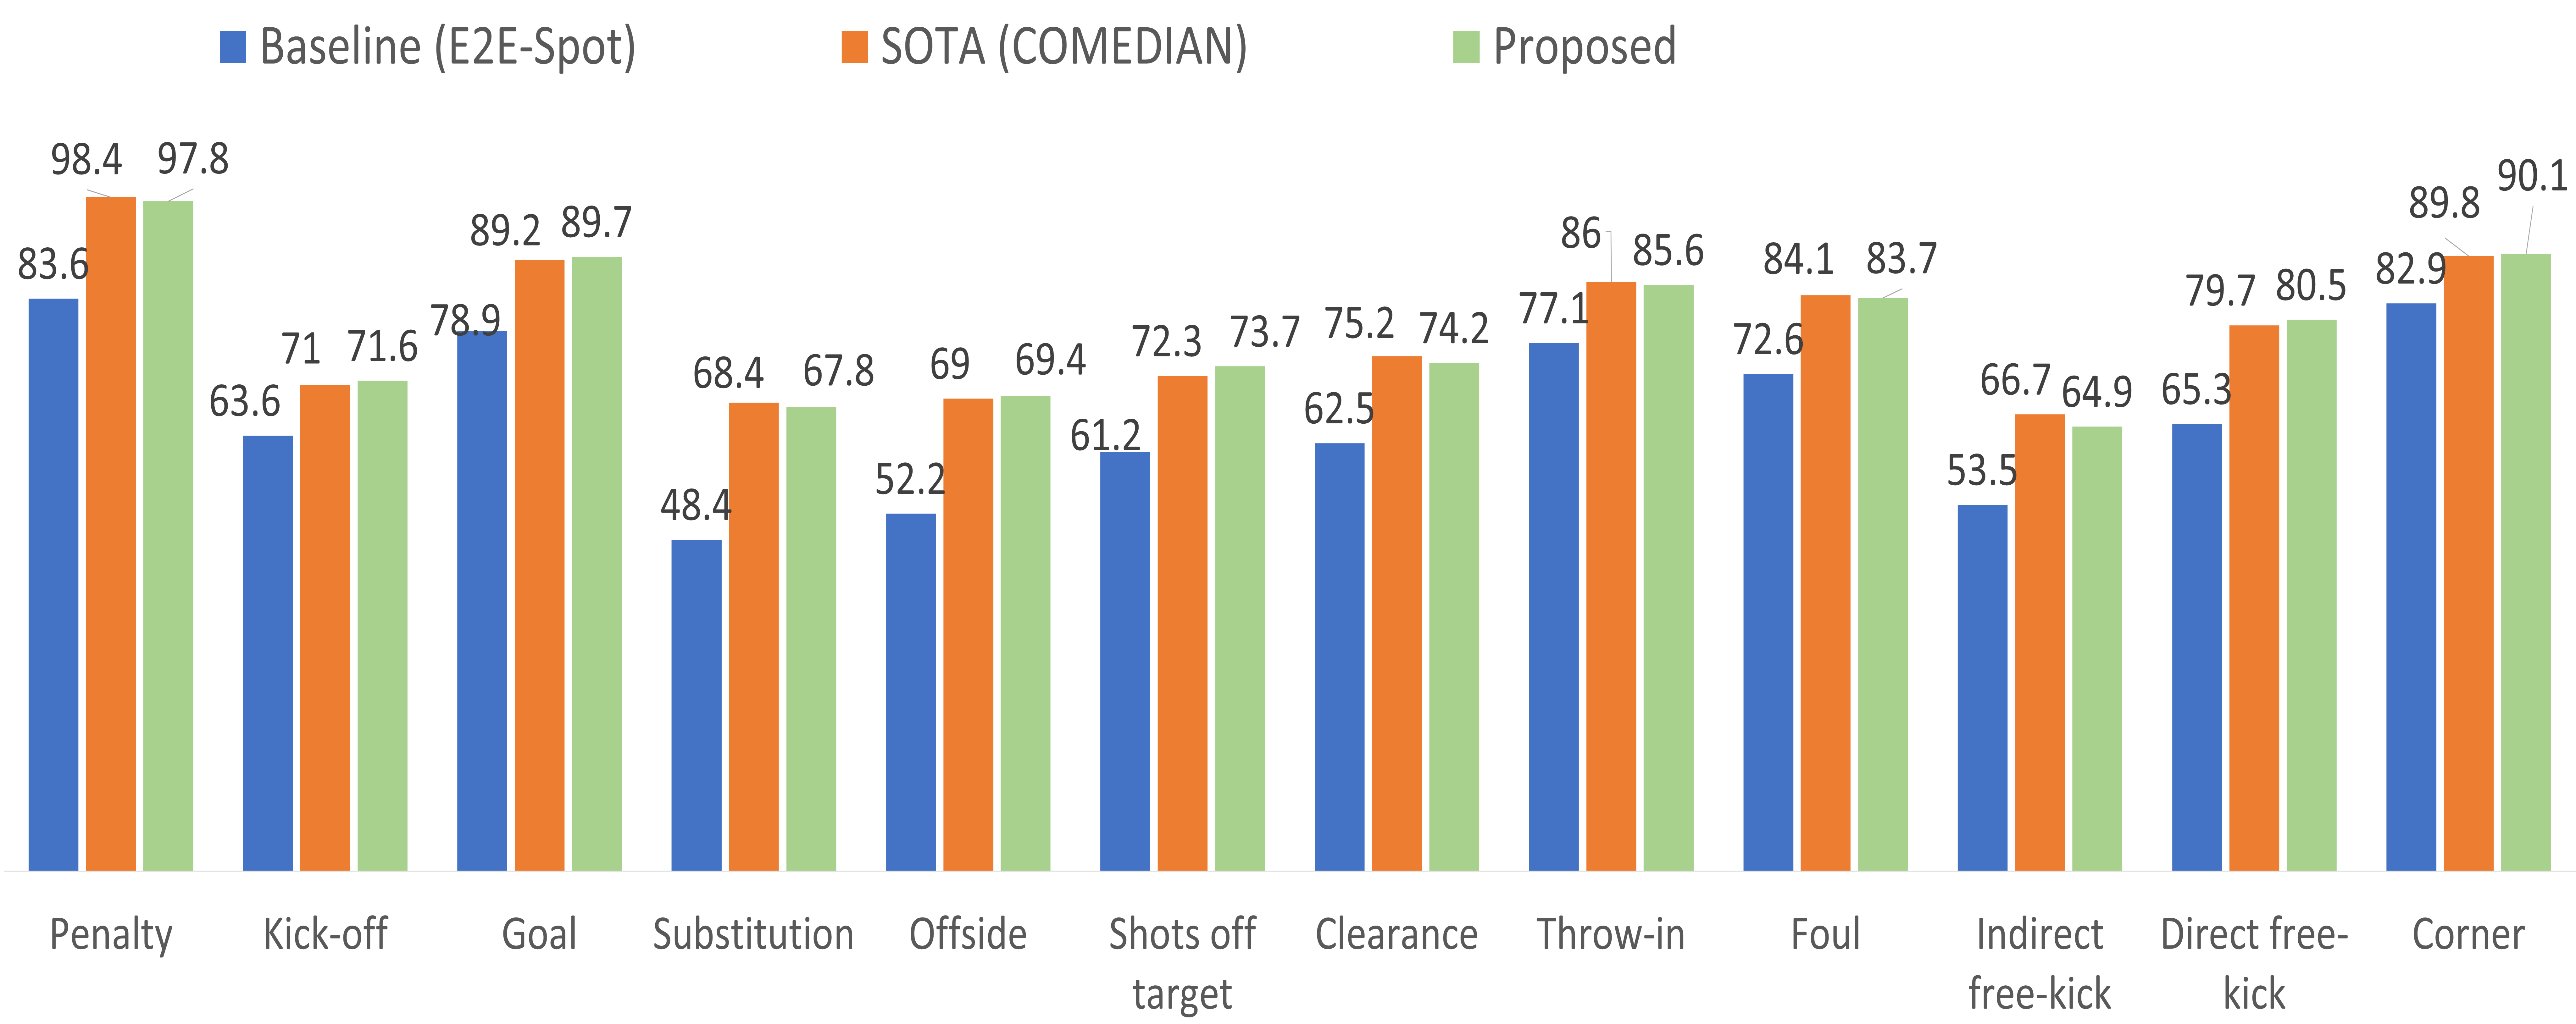}
    \caption{Per-class score comparison on tight setting in terms of \textbf{mAP} on few classes of SoccerNet V2 dataset.} \label{fig:per_soccer}
\end{figure*}
\begin{figure}[t!]
\subfloat[Tennis dataset~\cite{vid2player}]{\centering
    \includegraphics[width=0.49\textwidth]{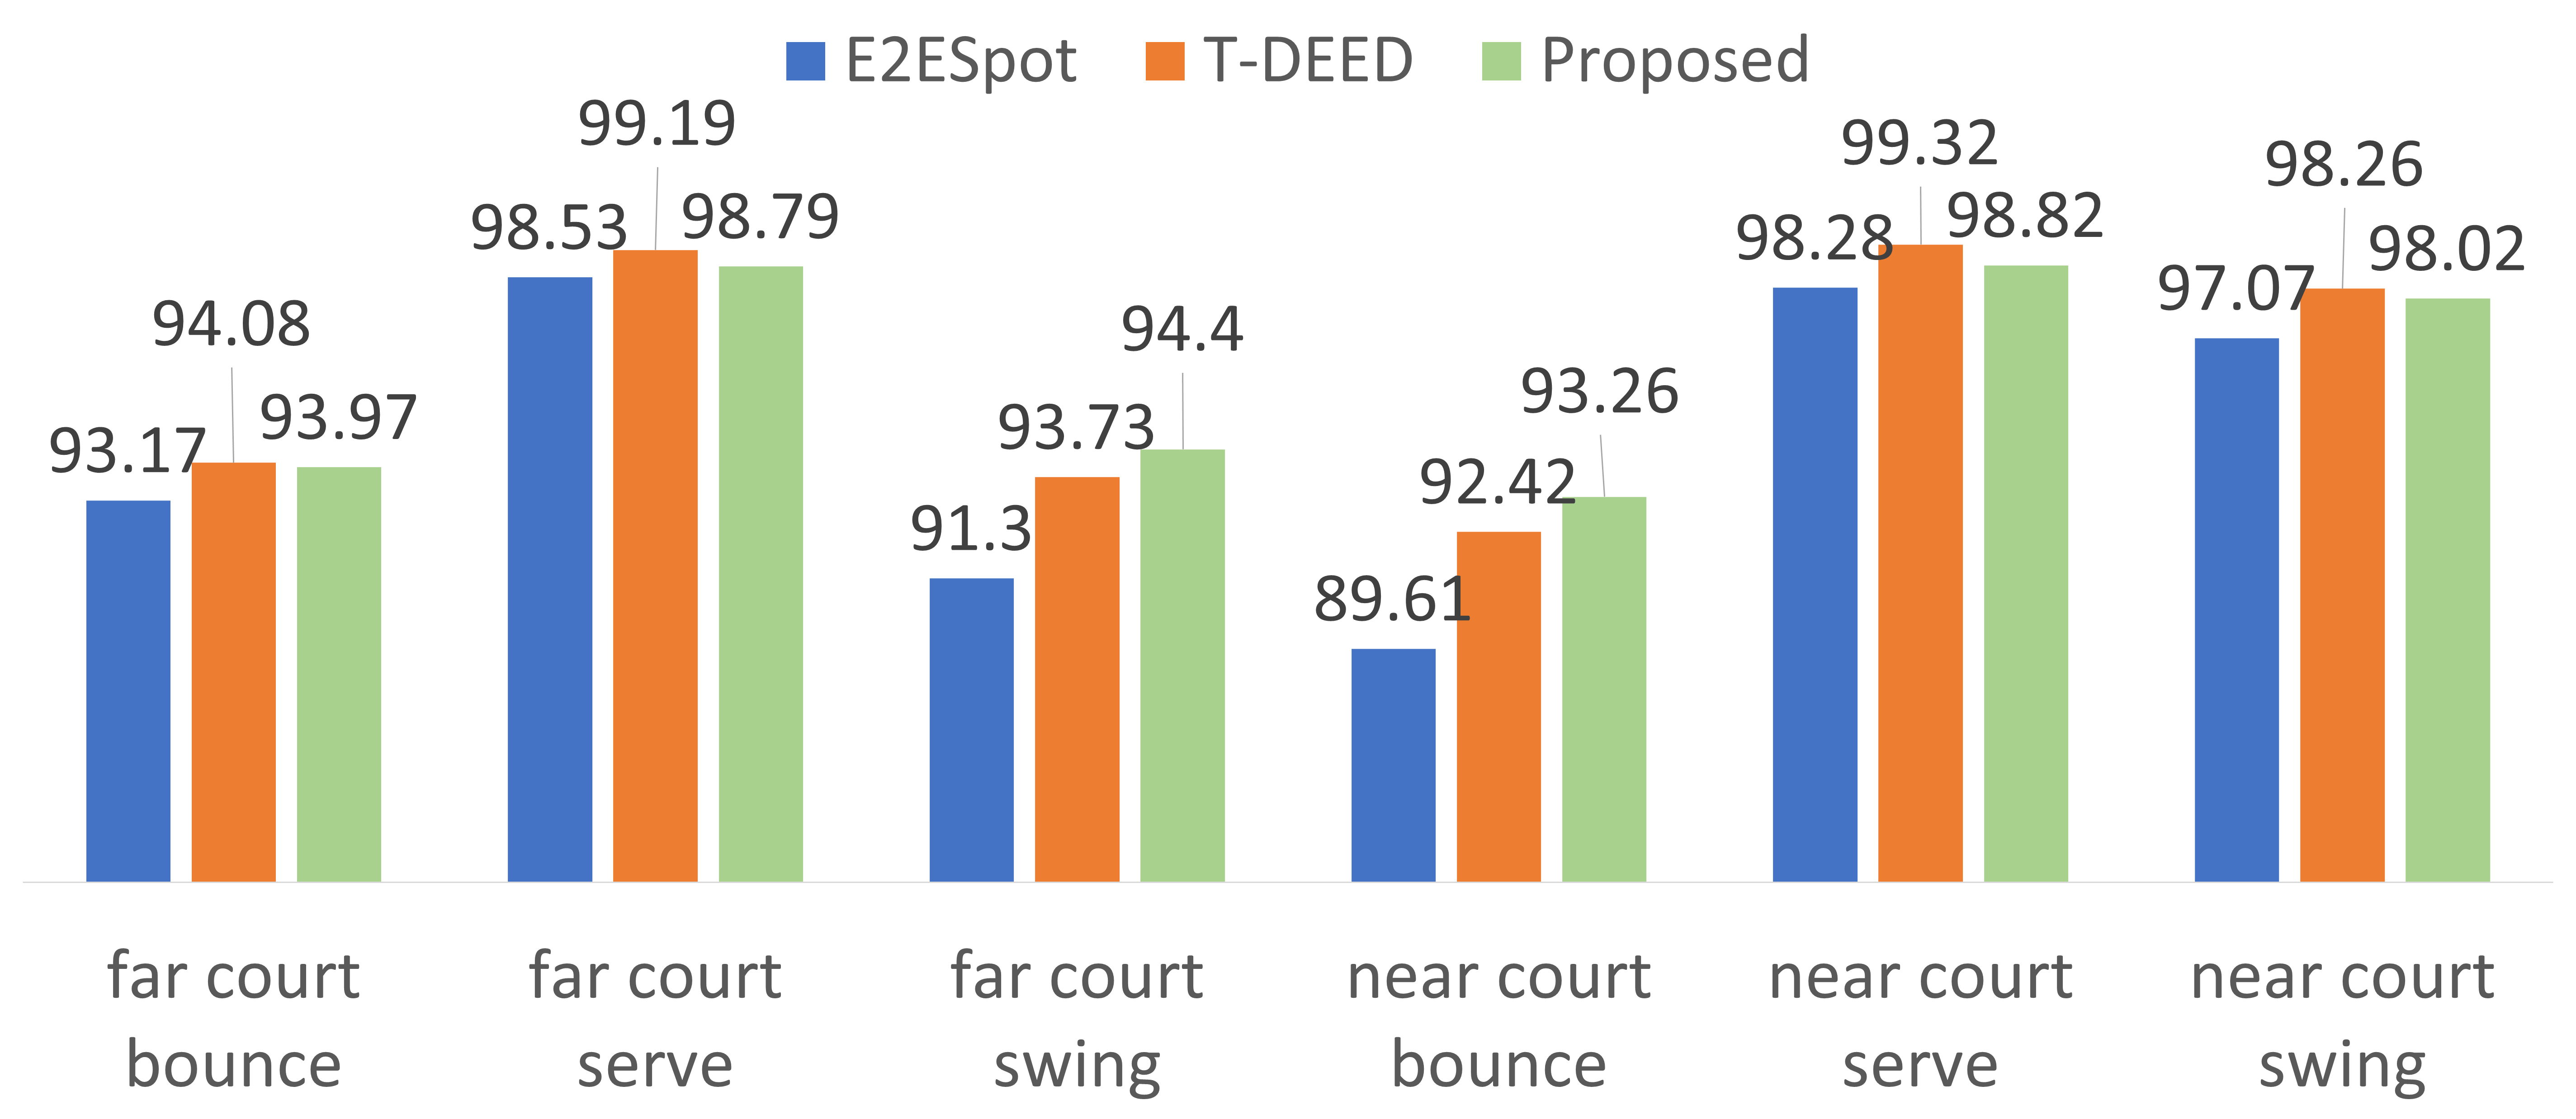}}\\
\subfloat[FS-Comp dataset~\cite{fs}]{\centering
    \includegraphics[width=0.49\textwidth]{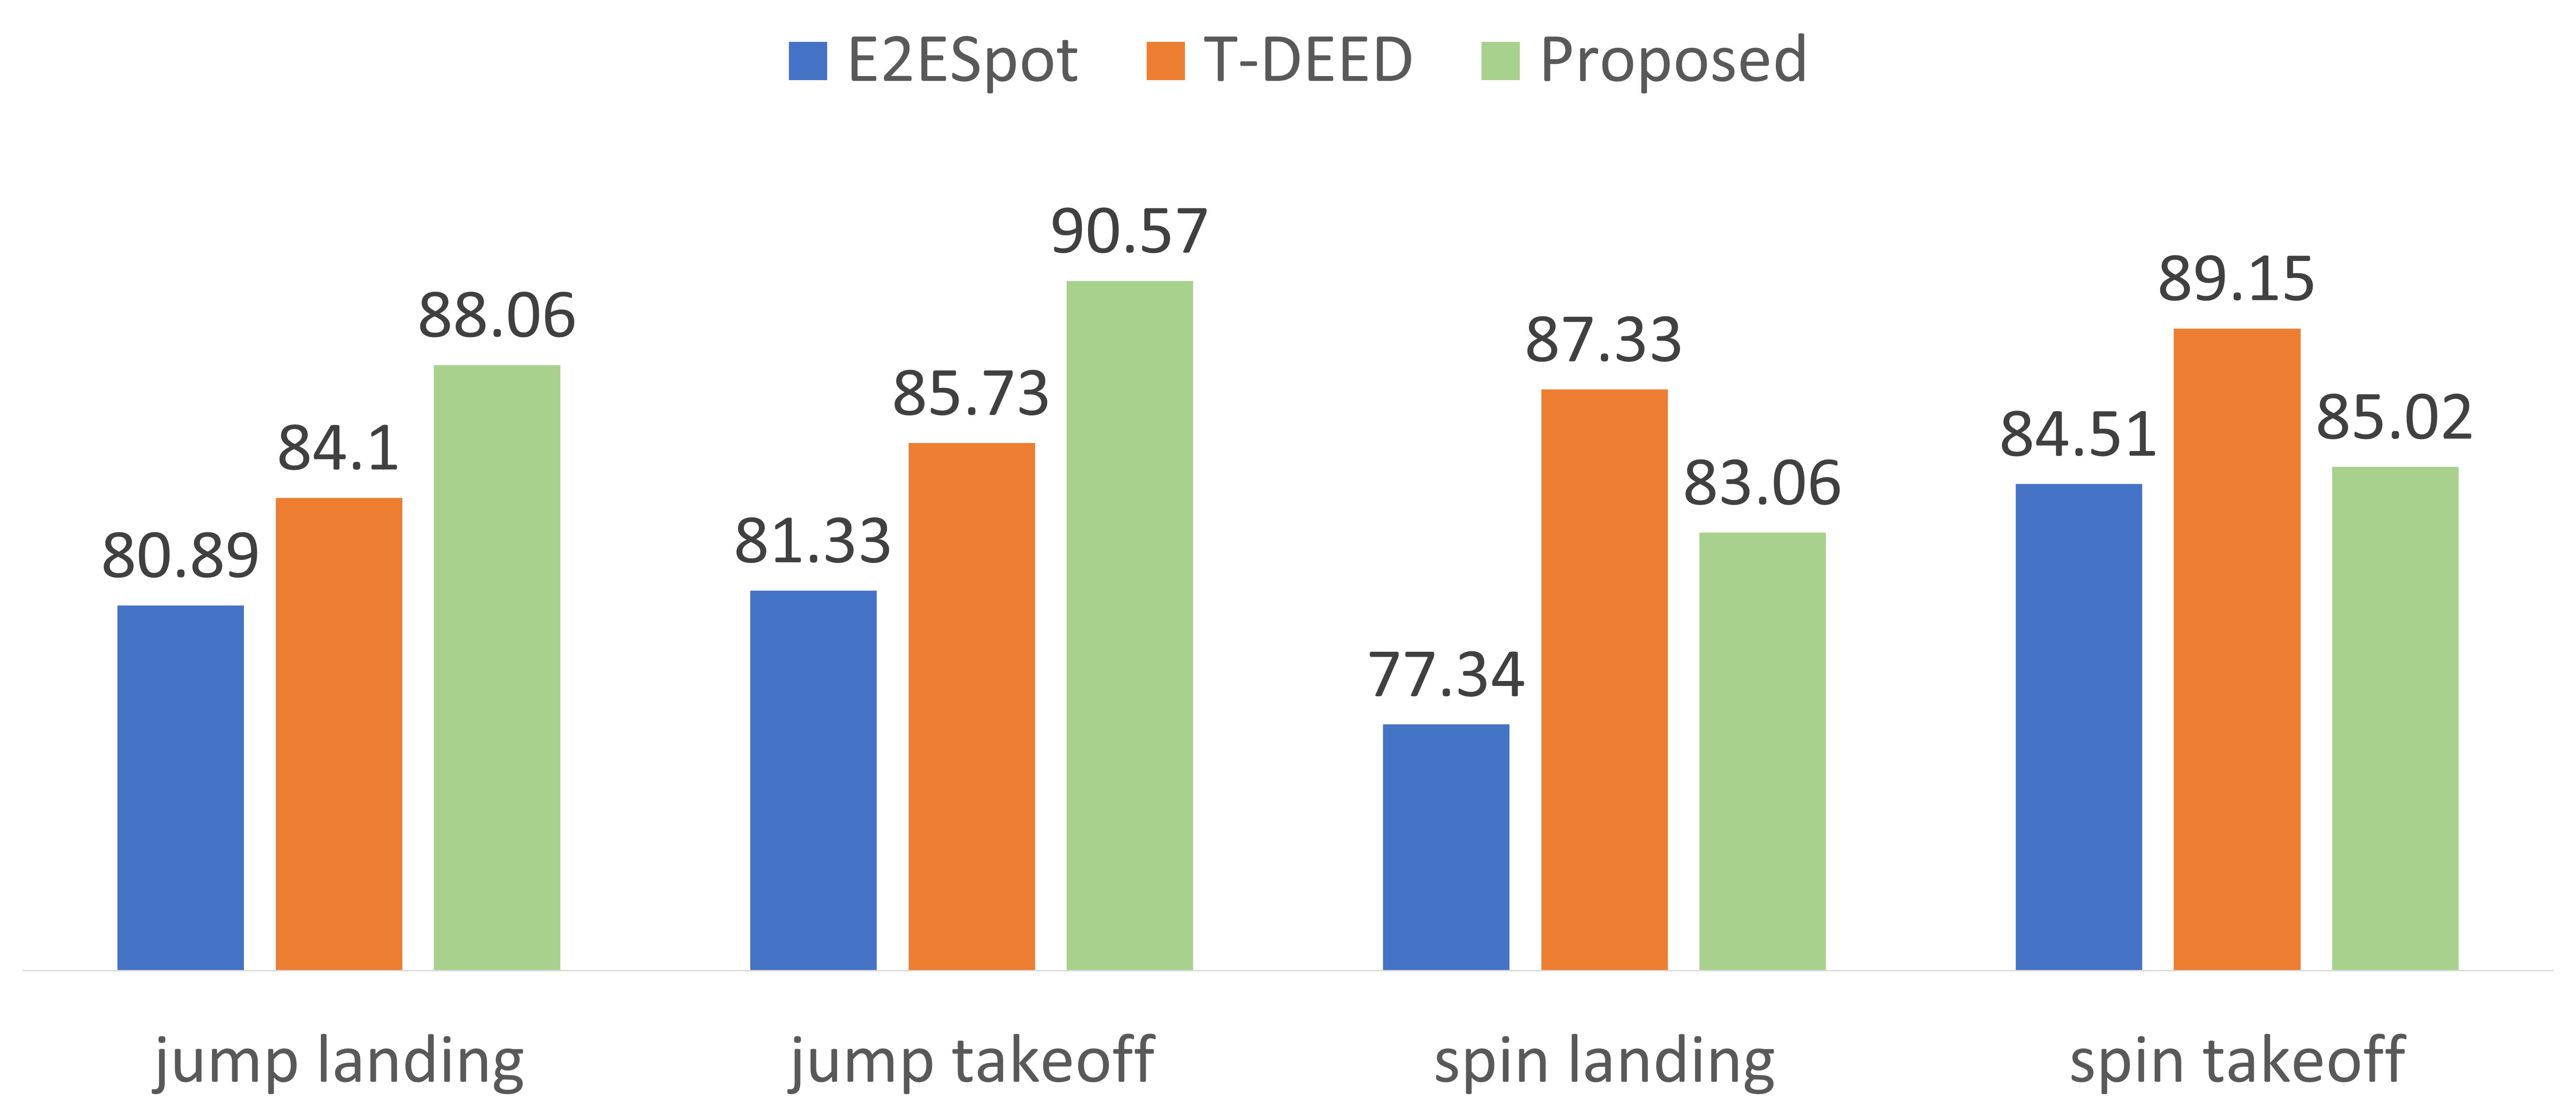}}\\
\subfloat[FS-Perf dataset~\cite{fs}]{\centering
    \includegraphics[width=0.49\textwidth]{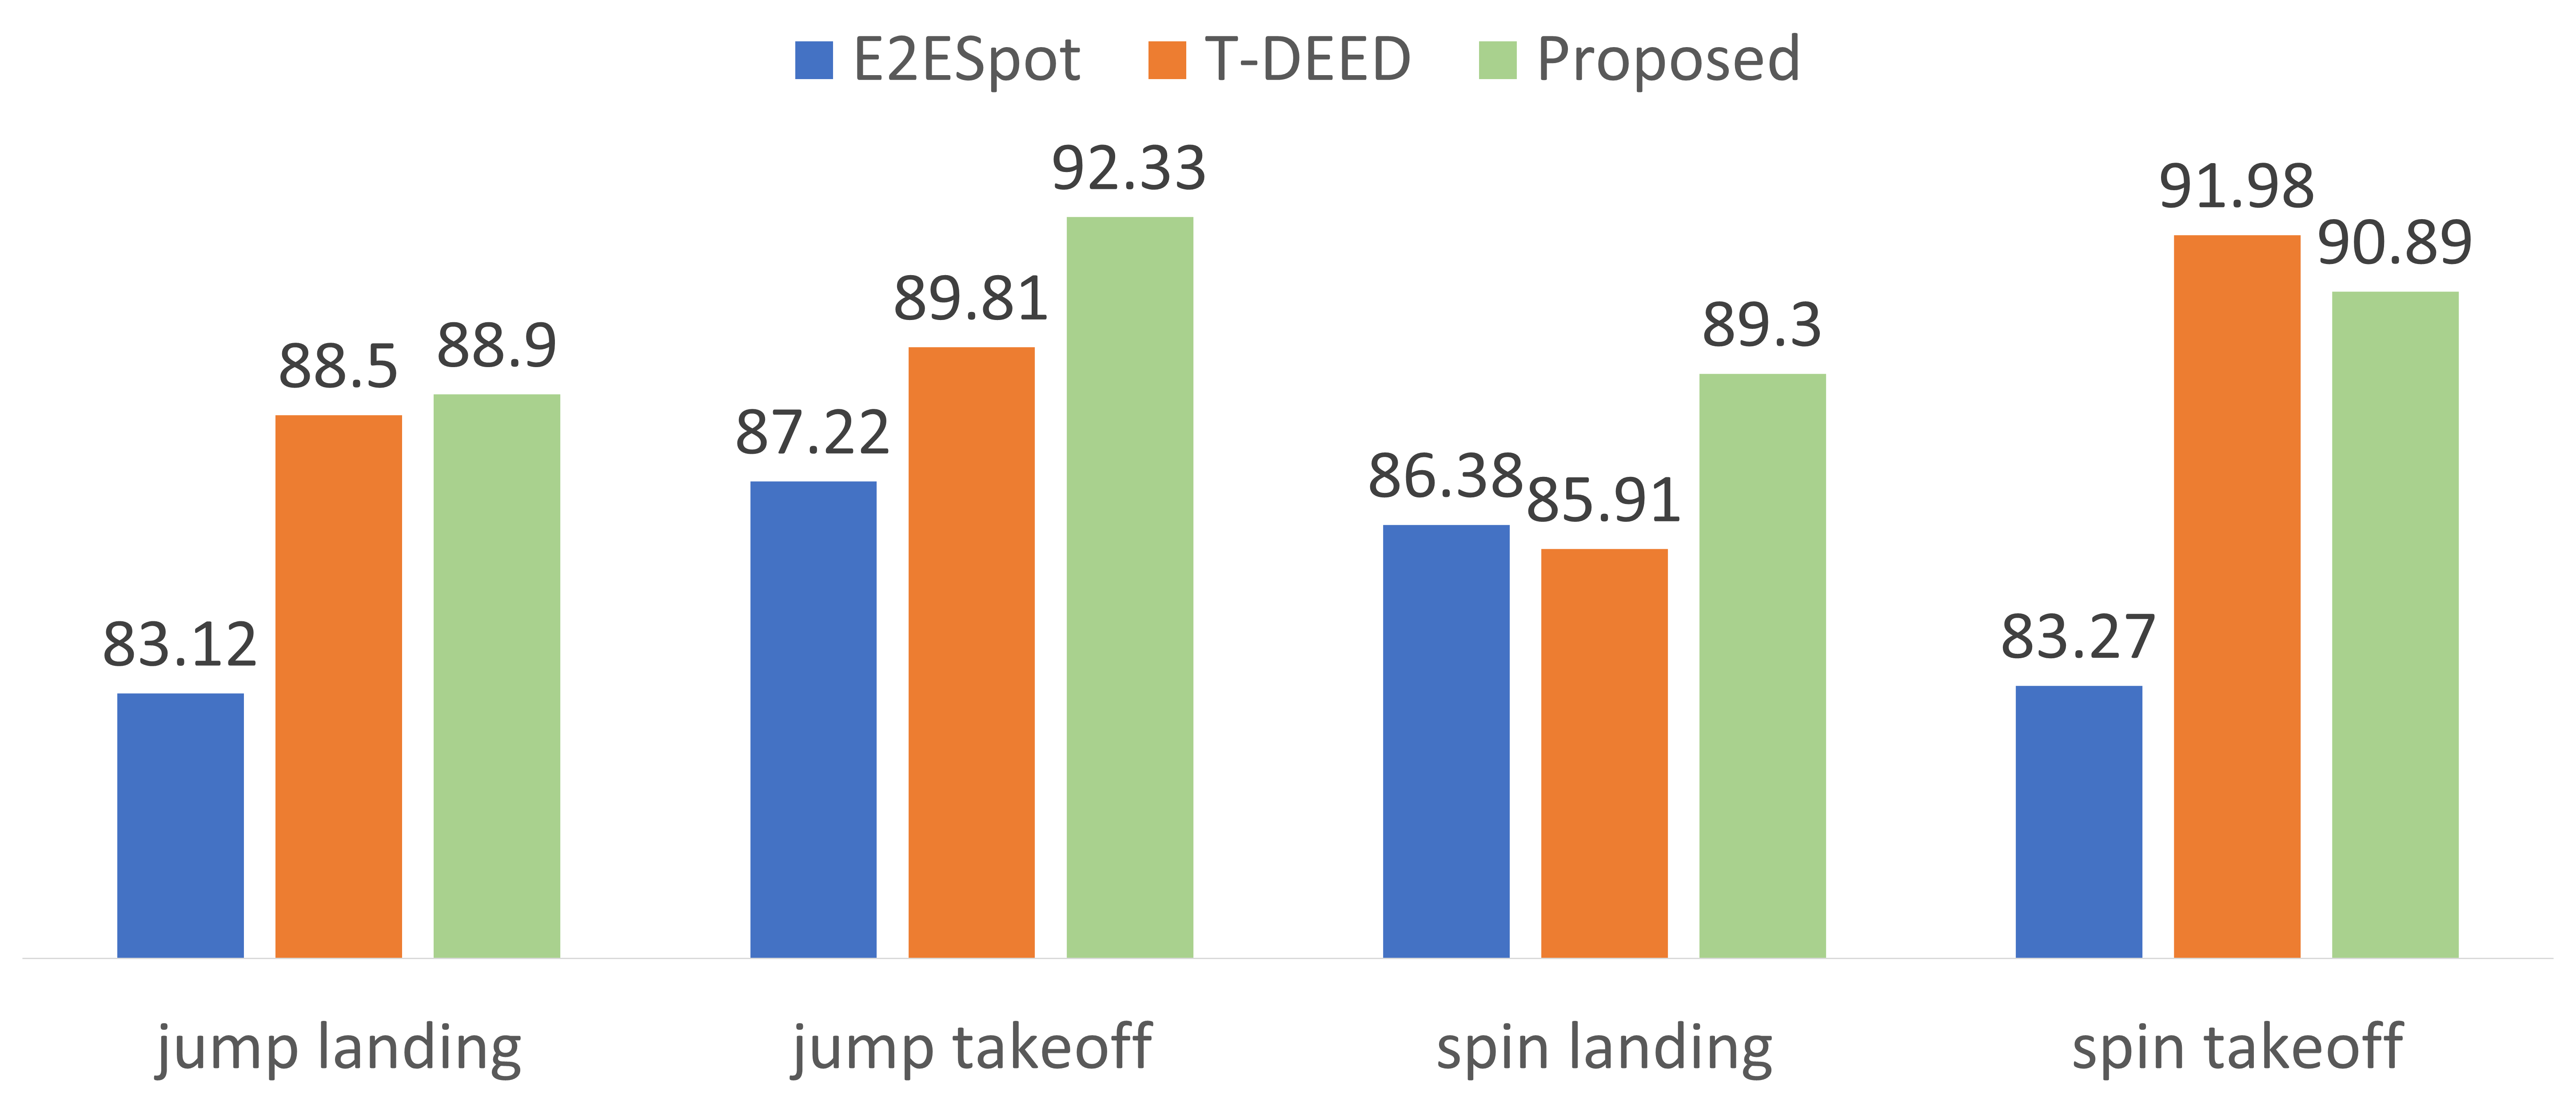}} \\
    \caption{Per-class score comparison on $\delta=1$ in \textbf{mAP} on Tennis and Figure Skating (i.e., FS-Comp \& FS-Perf) datasets.}
    \label{fig:per_class_tennis_fs}
\end{figure}

\begin{figure*}[t!]
    \includegraphics[width=\linewidth]{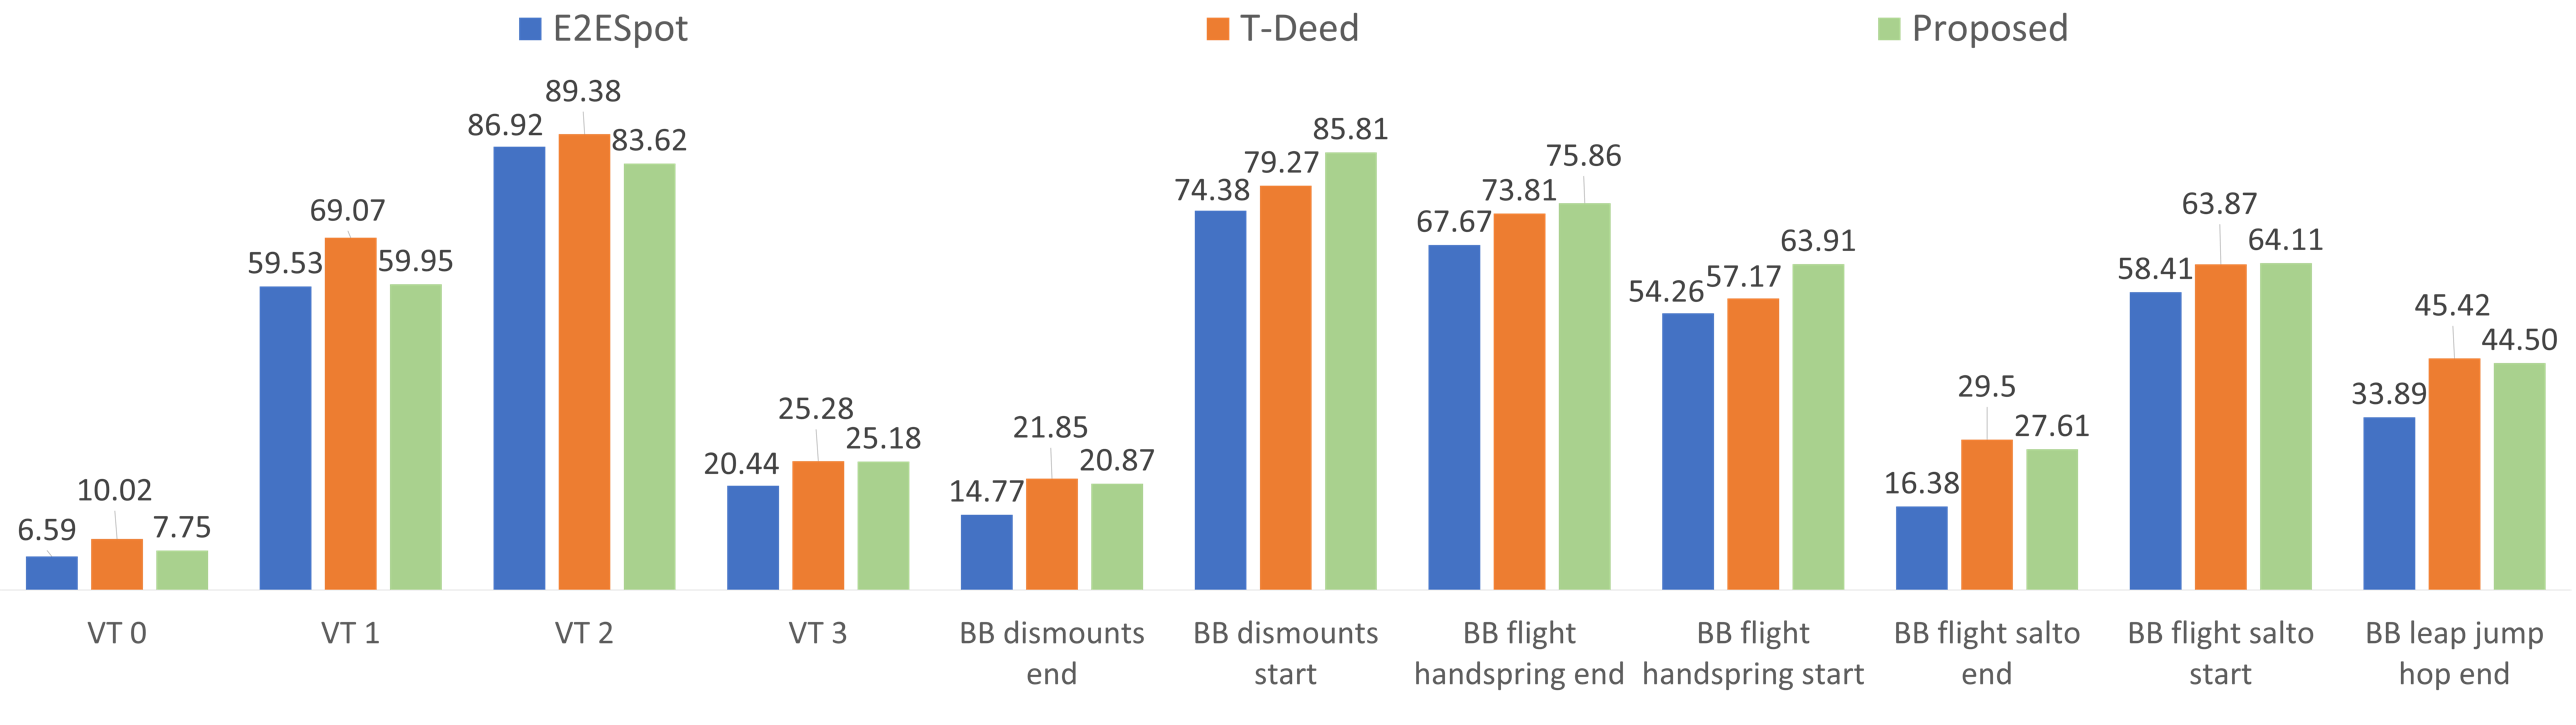}
    \includegraphics[width=\linewidth]{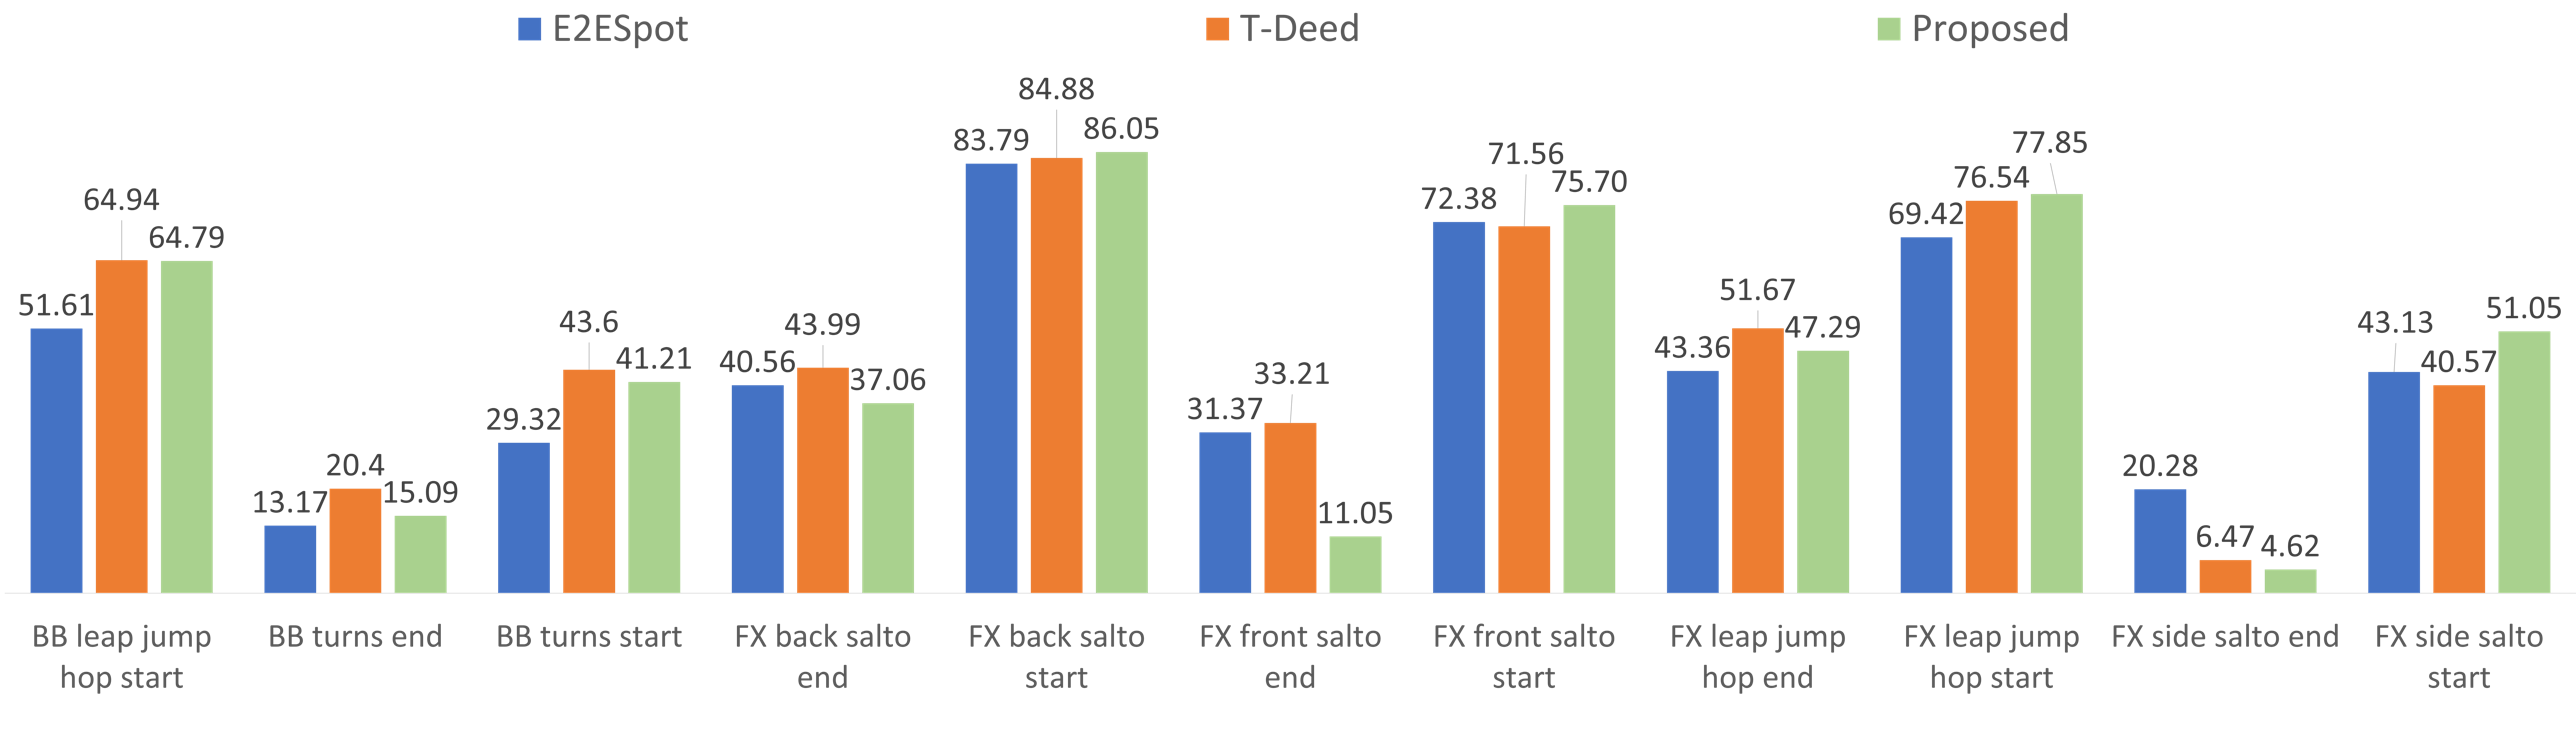}
    \includegraphics[width=\linewidth]{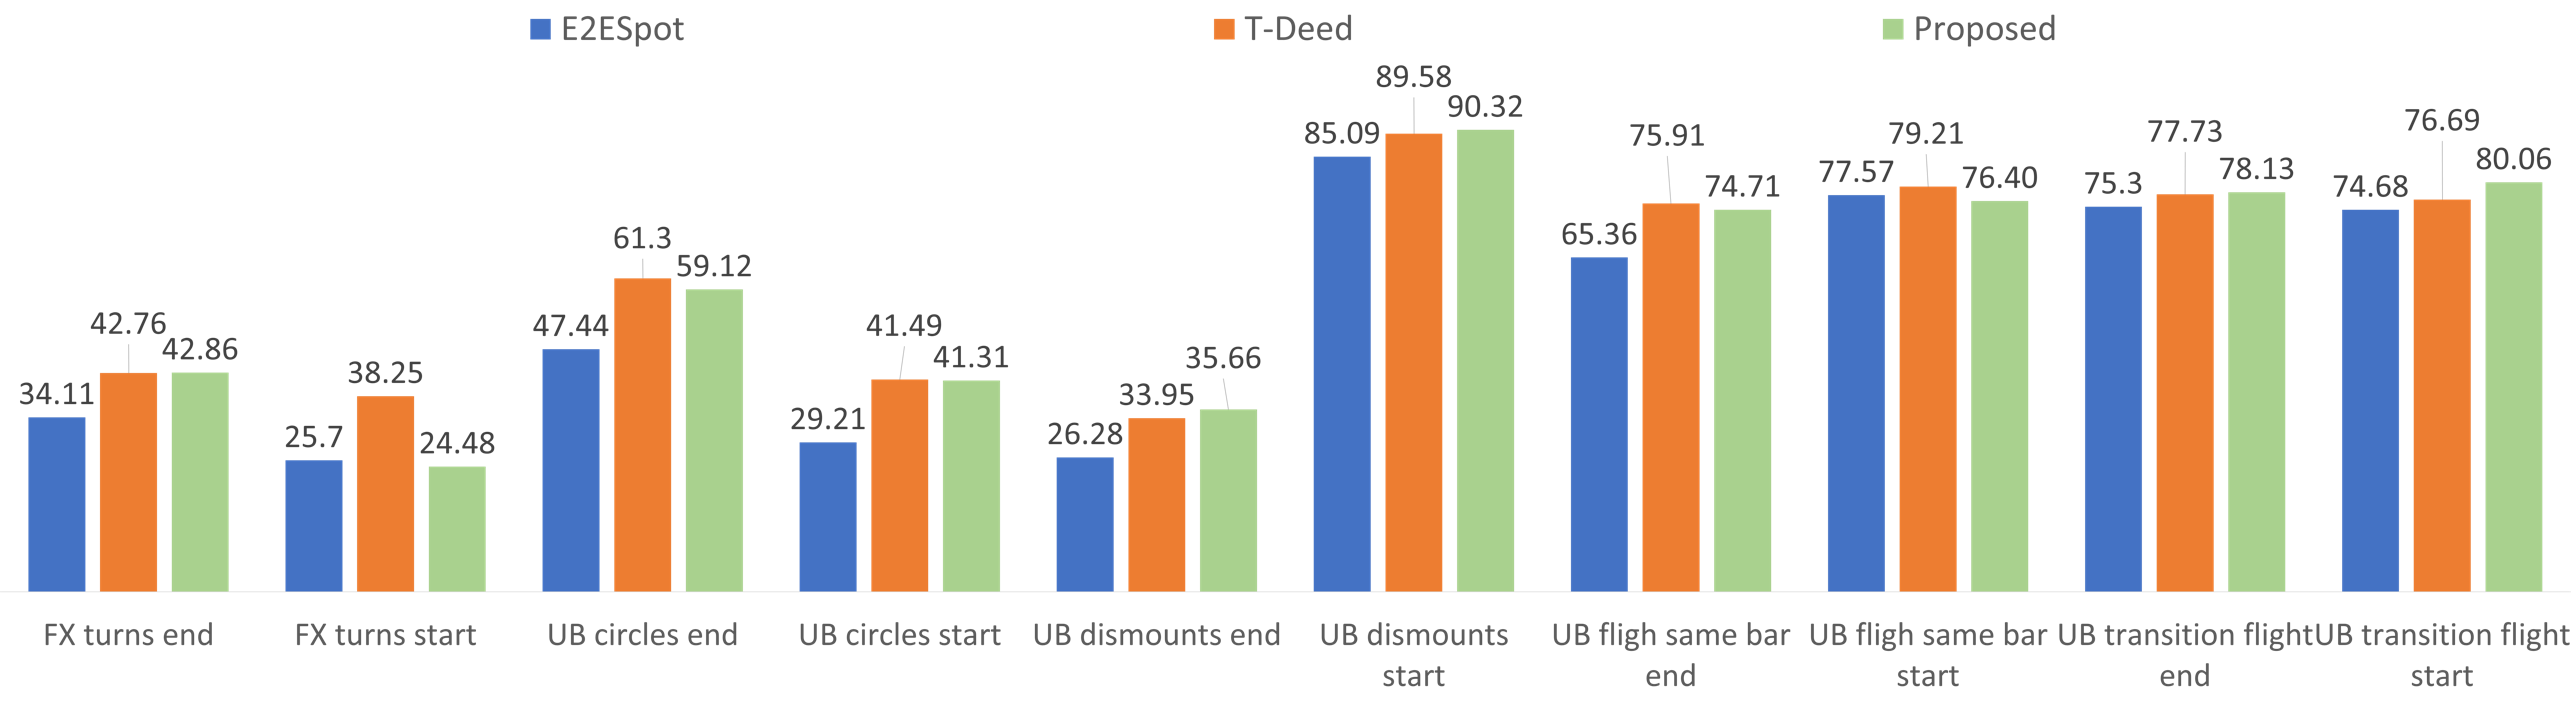}
    \caption{Per-class score comparison on $\delta=1$ in \textbf{mAP} on FineGym~\cite{finegym} dataset. Graph split on multiple rows for better visualization.} \label{fig:per_finegym}
\end{figure*}

% Parameter count comparison
\section{ Efficiency Comparison}
This paper demonstrates that our proposed method outperforms existing SOTA methods, especially in tight settings with a simpler network architecture. Here we have quantitatively validated this claim in detail.
In Table~\ref{tab:efficiency}, we provide a quantitative analysis of its efficiency, specifically in terms of the number of parameters and the computational complexity measured in GFLOPs. For a fair comparison, all the calculations are done from the models on their respective repo with an input size of $3\times 100\times 224\times 398$.
Our proposed method requires 77.49 GFLOPs and 6.46 million parameters, showcasing a substantial reduction in both computational complexity and model size compared to recent SOTA methods \cite{comedian, yahoo-icip, astra, e2espot, T-DEED} except E2E-Spot (RegNet-Y 200MF) \cite{e2espot} and T-DEED (RegNet-Y 200MF) \cite{T-DEED}. Among them, only COMEDIAN (ViSwin) \cite{comedian} achieves comparable results but with a significantly larger number of parameters and higher computational requirements. Similarly, the Spivak~\cite{yahoo-icip} and ASTRA~\cite{astra} achieve similar results only in the loose-mAP setting, even with increased parameters.

E2E-Spot (RegNet-Y 200MF), T-DEED (RegNet-Y 200MF), and our proposed method utilize similar structured networks, but some modules differ. Consequently, the proposed method has a higher number of GFLOPs than both methods. While, the T-DEED (RegNet-Y 200MF) has a significantly larger number of parameters than the proposed method. Nonetheless, our proposed method outperforms both methods significantly.
This balance between efficiency and performance is crucial for practical applications, particularly in environments with limited computational resources. This makes it an appealing choice for real-world deployments where both computational efficiency and high performance are essential.

\section{ Per Class Score Comparison}
\label{sec:per_class_score}
In addition to the per-class score analysis shown in Figure 1 and Figure 4 in the main manuscript, we have included some additional analyses. Specifically, in Figure~\ref{fig:per_soccer}, we have presented the tight-mAP scores of the SoccerNet V2 dataset for classes that were not covered in Figure 1 of the main paper. Additionally, Figure~\ref{fig:per_class_tennis_fs} presents the per-class score analysis on $\delta=1$ setting for the Tennis and Figure Skating (FS-Comp and FS-Perf) datasets.

In Figure~\ref{fig:per_soccer}, it is evident that the proposed method achieves comparable performance with COMEDIAN~\cite{comedian} method despite having significantly fewer parameters and lower computational complexity. While from Figure~\ref{fig:per_class_tennis_fs} and Figure~\ref{fig:per_finegym} it can be observed that the proposed method achieves comparable performance in most of the classes while outperforming the T-DEED \cite{T-DEED} in many instances. 

% the proposed method outperforms other methods, except for ``near court serve'' in the Tennis dataset, ``spin landing'' and ``spin takeoff'' in the FS-Comp dataset, and ``spin takeoff'' in the FS-Perf dataset, where the proposed method achieves comparable results with the SOTA method \cite{T-DEED}.

\section{ Limitations}
In the main manuscript, we noted that our proposed method is focused on sports events, which may give the impression of limited applicability. However, it is essential to clarify that none of the components of our method are specifically designed for sports videos. The concept of precise event spotting has mainly been defined in relation to sports, which is why the existing precise event spotting datasets predominantly consist of sports videos. The lack of datasets featuring non-sports videos is one reason we cannot claim that our proposed method also applies to non-sports data. Furthermore, events are typically defined by specific starting and ending times and rarely occur instantaneously. Although we could approach the problem as detecting the precise start and end times of events, current temporal action detection datasets may not be suitable for this purpose. They require extensive preprocessing before they can be effectively utilized.
